# Supplementary material for: The Data Enclave Advantage: A New Paradigm for Least-Privileged Data Access in a Zero-Trust World
Source: arXiv:2510.09494 source file (2025-10-10)
Supplement: Supplementary file 1 [file appendix.tex]

\section{Appendix}
